# Supplementary material for: Lattice-Driven Chiral Charge Density Wave State in 1T-TaS$_{2}$
Source: arXiv:2112.03367 source file (2021-12-06)

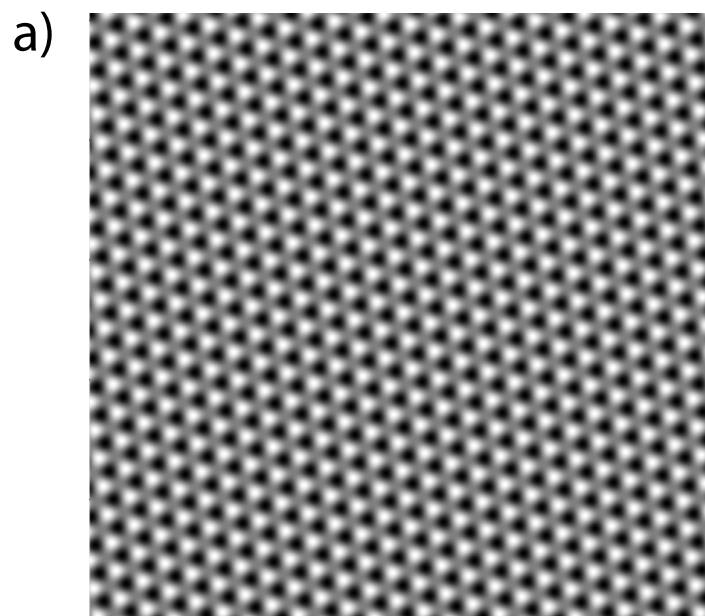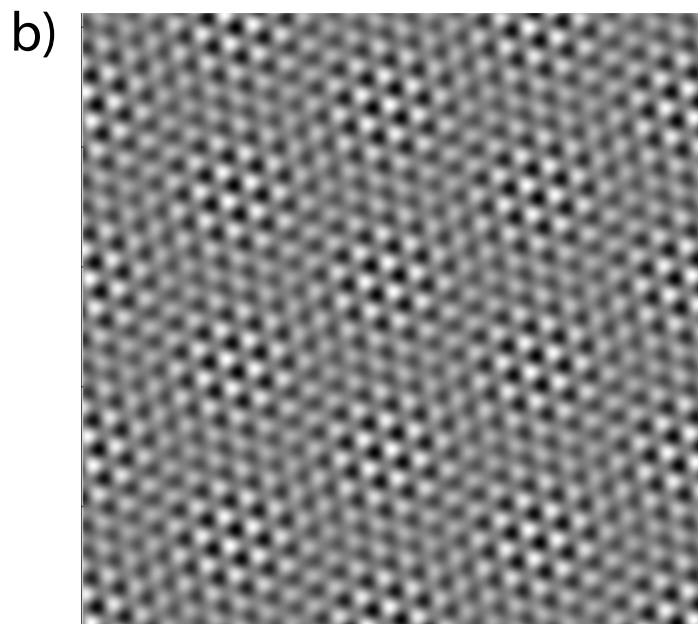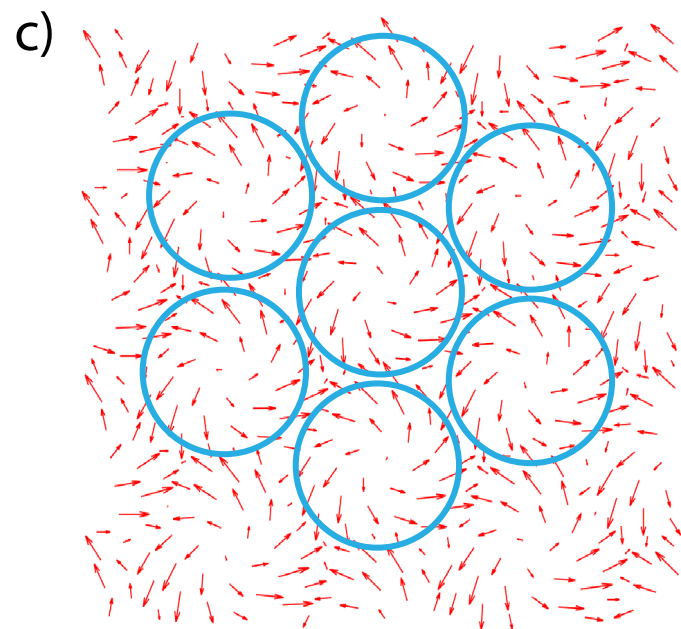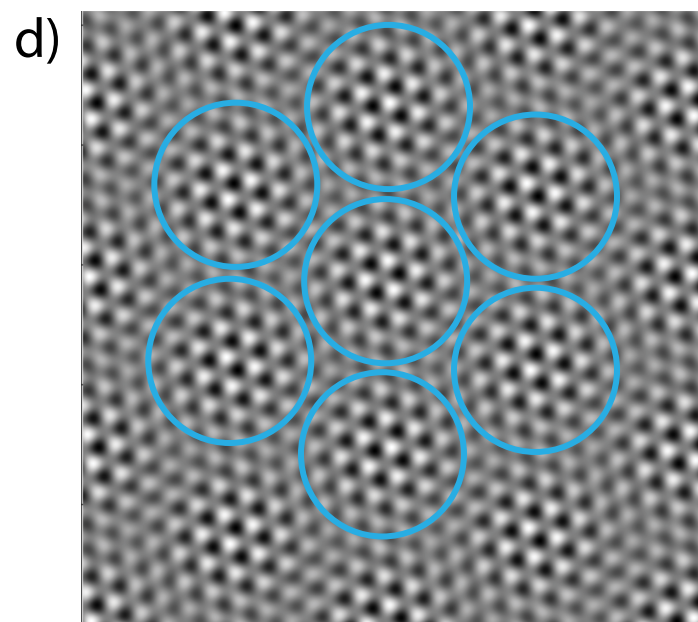

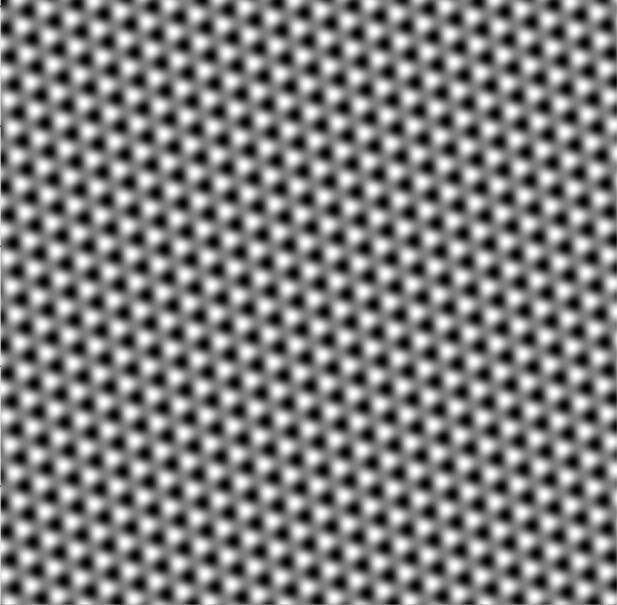

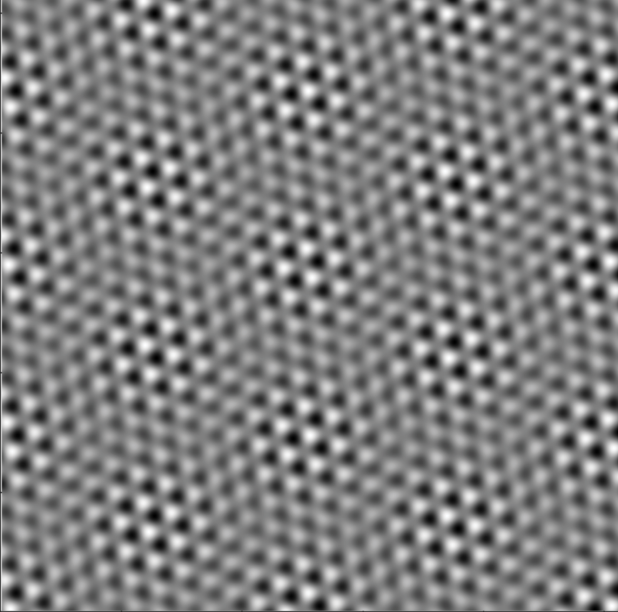

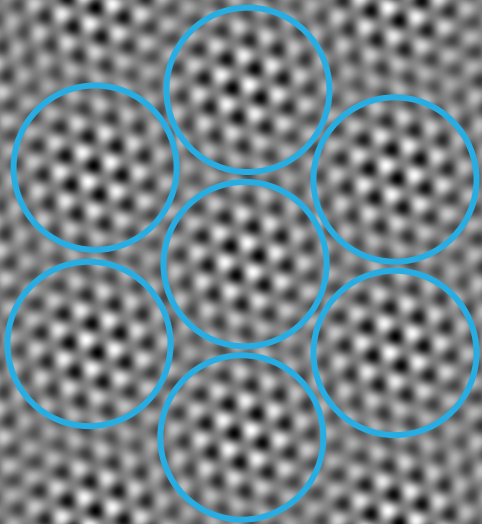

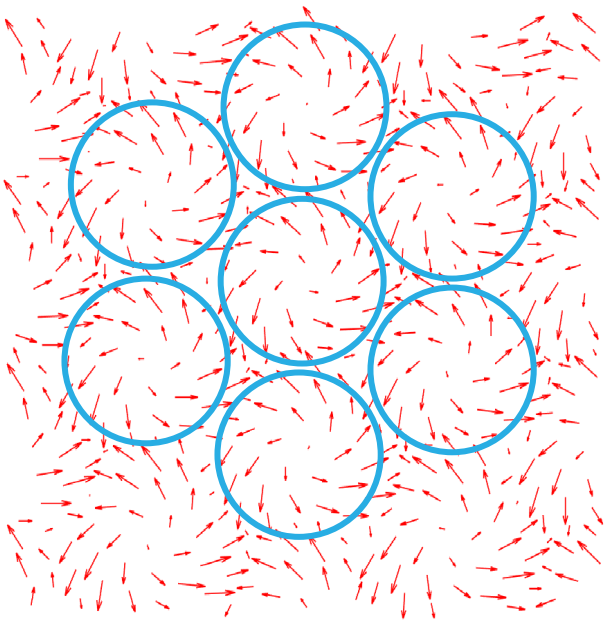

Supplement: Supplementary file 1 [file TaS2_SupMat.pdf]
